# Supplementary material for: An HCI View of Configuration Problems
Source: arXiv:1601.01747 source file (2016-01-08)
Supplement: Supplementary file 1 [file appendix.tex]

\subsection{A. Characteristics of Dataset}

Table~\ref{tab:scale} shows the scale of ServerFault.com (SF) and StackOverflow.com (SO) 
in terms of user base, posts, and tags. The numbers indicate that system
administration is a much smaller community compared with programming\footnote{Given SF and SO
are within the same Q \& A network with the same vendors, we assume that they have the similar visibility.}. 
Please note that configuration errors might have similar level of severity as software defects. 

\begin{table}[ht]
\caption{Comparison of SF and SO} % title of Table
\centering % used for centering table
\small
\begin{tabular}{l | c c } % centered columns (4 columns)
\hline
Q \& A site     &      ServerFault.com    &      StackOverflow.com  \\
\hline
Users           &      129,155             &      2,305,505        \\
Posts           &      162,667             &      6,186,948        \\
Tags            &      5,292               &      36,918           \\
\hline
\end{tabular}
\label{tab:scale} % is used to refer this table in the text
\end{table}

Figure~\ref{fig:tags} shows the top 20 tags with the most numbers of posts on SF.
Eight of them, including No. 1 tag ``linux,'' are tags operating systems acting as
the infrastructure running software to provide utilities and services\footnote{Linux beats Windows 
as the major platform for system services (oh, yeah)!}. Most posts
with OS tags are not related to OS kernels but the software running upon it such
as web servers and database servers. This is the reason we do not pick OS in our study.
From Figure~\ref{fig:tags}, we can see that ``apache2'' is the No. 2 tag and is a tag
for a single, special software, so we pick Apache HTTP server as our target software.

\begin{figure}[tb!]
\centering
\includegraphics[width=0.45 \textwidth]{tag_pop}
\caption{Top 20 tags with the most numbers of posts. Apache is the most posted tag of a single software.}
\label{fig:tags}
\end{figure}

Figure~\ref{fig:num_posts} shows the number of posts tagged with ``apache2'' on SF in the time series
from the first month it was launched (Apr. 2009) till time we crawled the website (Oct. 2013). In our study, we 
only examine the posts with answers accepted by the posters (the red bars in Figure~\ref{fig:num_posts}). 
Interestingly, for some reasons, more and more posts on SF remains unanswered (the yellow bars) with the time increasing
(while the total number of posts do not vary significantly).

\begin{figure}[tb!]
\centering
\includegraphics[width=0.45 \textwidth]{timeseries}
\caption{Number of posts tagged with ``apache2'' on ServerFault.com. Our examined cases
are randomly sampled from the red area (i.e., cases with accepted solutions).}
\label{fig:num_posts}
\end{figure}

\subsection{B. Analysis on Correlated Tags}

Figure~\ref{fig:coexist_tags} shows the tags most coexisting with the ``apache2'' tag we study
in this paper. We can see that among the top 20 tags 40\% of them are built-in modules or features of 
Apache web server (e.g., mod-rewrite, redirect), 20\% are other software used together with
Apache (e.g., php, mysql), and 20\% are OS platforms (e.g., linux, centos).
Apache is typically used as a building component of a LAMP (Linux, Apache, MySQL, and PHP) stack, 
a free and open-source software solution for high-availability heavy-duty dynamic websites.
Figure~\ref{fig:lamp} shows one typical example of LAMP together with Ngnix used as a proxy. This explains
the strong correlation with tags ``linux,'' ``nginx\footnote{Another reason for the correlation 
of Apache and Ngnix is that both of them are popular web servers, and are frequently compared and discussed.} ,'' ``php,'' and ``mysql.''

\begin{figure}[tb!]
\centering
\includegraphics[width=0.45 \textwidth]{tags_apache}
\caption{Top 20 tags correlated with ``apache2.'' {\bf 40\%} of them are modules (features)
         of Apache web server, {\bf 20\%} are other software commonly used together with 
         Apache, and {\bf 20\%} are the platform running Apache.}
\label{fig:coexist_tags}
\end{figure}

\begin{figure}[tb!]
\centering
\includegraphics[width=0.35 \textwidth]{lamp}
\caption{An example of the LAMP stack}
\label{fig:lamp}
\end{figure}

\subsection{C. The Configuration Activity Model}

Figure~\ref{fig:act_model} demonstrates the activity model of performing configuration tasks.
Before zooming into details and setting configuration parameters, system administrators first
need to select the proper software (e.g., Linux or Windows) or a combination of software (e.g., LAMP),
as well as to read user manuals or tutorials in order to understand basic concepts and 
configuration requirements (e.g., formats, constraints). During these processes, 
sysadmins collect knowledge and nail down to specific, concrete configuration tasks 
(e.g., which file to edit, which parameter to set).

If the sysadmin's configuration solution does not result in a working system (i.e., containing errors),
she needs to change her configuration settings by fixing the {\it active errors} until the system
behavior matches her expectation. Here, {\it active errors} refers to the situation that the sysadmin knows
the error and try to fix the error. After the system works correctly, she might further
try to test/validate whether the working system can handle all possible system inputs (e.g., workloads). 

When a working system encounters failures or anomalies due to workload changes or latent errors (errors
that did not manifest in the first place), the sysadmin needs to diagnose the failure ---locating the
error based on its manifestation (e.g., failure stacks, error logs). When the sysadmin figures out the
root cause in terms of the errors inside her configuration settings, the latent error becomes an active
error. The procedure falls into the previous ones. 

\begin{figure}[tb!]
\centering
\includegraphics[width=0.45 \textwidth]{activity_model}
\caption{The activity model of a configuration process}
\label{fig:act_model}
\end{figure}

\subsection{D. Nielsen's 10 Heuristics for User Interface Design}

Heuristic evaluation~\cite{nielsen:90,nielsen:94} is a usability engineering method for 
finding the usability problems in a user interface design so that they can be attended to 
as part of an iterative design process. Heuristic evaluation involves having a small set of evaluators 
examine the interface and judge its compliance with recognized usability principles (the ``heuristics''). 

Table~\ref{tab:heuristics} shows the 10 most general heuristics for interface design. 
They are called ``heuristics'' because they are more in the nature of rules of thumb than specific usability guidelines.

\begin{table}[ht]
\caption{10 Heuristics for User Interface Design} % title of Table
\centering % used for centering table
\small
\begin{tabular}{ll c c c} % centered columns (4 columns)
    \hline
    \#  & Principles\\
    \hline
    \hline %inserts double horizontal lines
    1.  & Visibility of system status                   \\ % inserting body of the table
    2.  & Match between system and the real world       \\
    3.  & User control and freedom                      \\
    4.  & Consistency and standards                     \\
    5.  & Error prevention                              \\
    6.  & Recognition rather than recall                \\
    7.  & Flexibility and efficiency of use             \\
    8.  & Aesthetic and minimalist design               \\ %[1ex] % [1ex] adds vertical space
    9.  & Help users diagnose and recover from errors   \\
    10. & Help and documentation                        \\
    \hline %inserts single line
\end{tabular}
\label{tab:heuristics} % is used to refer this table in the text
\end{table}
